# Supplementary material for: Efficient Medical Image Assessment via Self-supervised Learning
Source: arXiv:2209.14434 source file (2022-09-28)
Supplement: Supplementary file 1 [file 09-appendix.tex]

\section{Appendix}

\subsection{Results on additional datasets - COVIDX~\footnote{\href{https://www.kaggle.com/andyczhao/covidx-cxr2?select=competition\_test}{https://www.kaggle.com/andyczhao/covidx-cxr2?select=competition\_test}}}
\label{app_data}
\vspace{-7mm}
\begin{figure}[h]
    \centering
    \subfloat[Add high value data]{
        \includegraphics[width=0.47\linewidth]{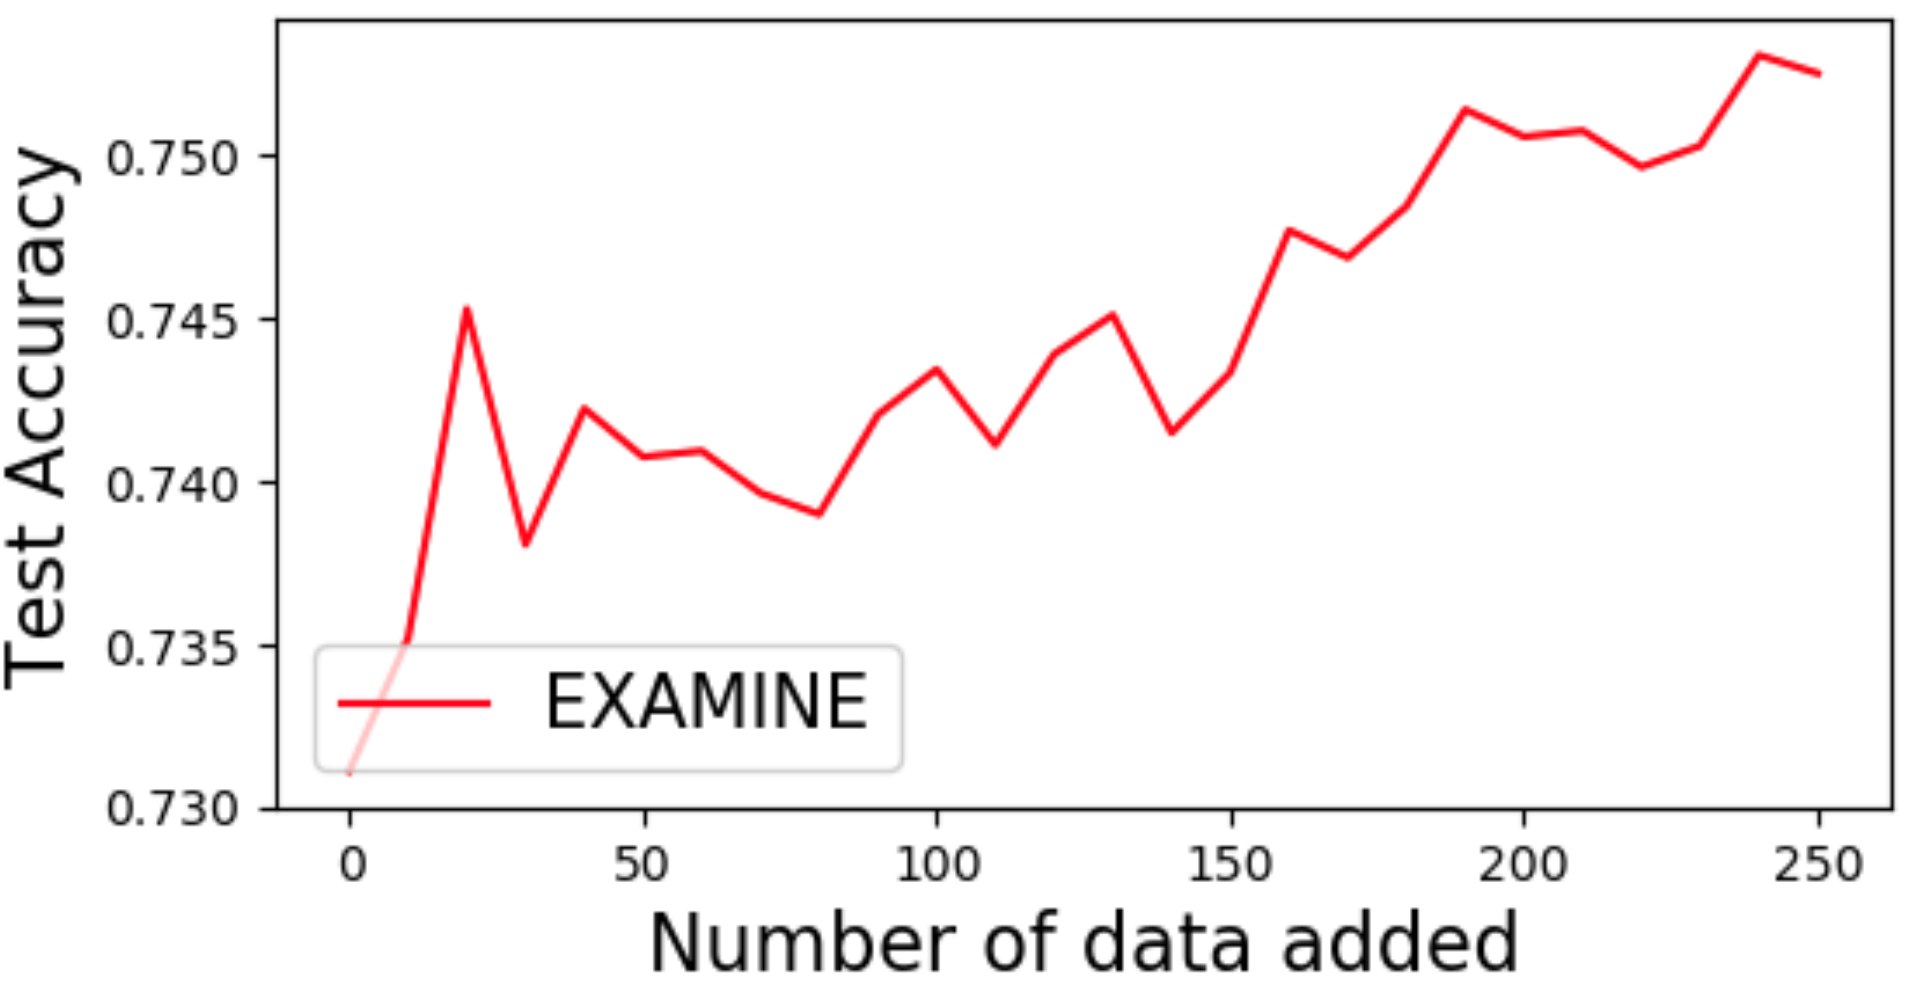}
        \label{fig:covidx_add_good}
    }
    \subfloat[Add low value data]{
        \includegraphics[width=0.47\linewidth]{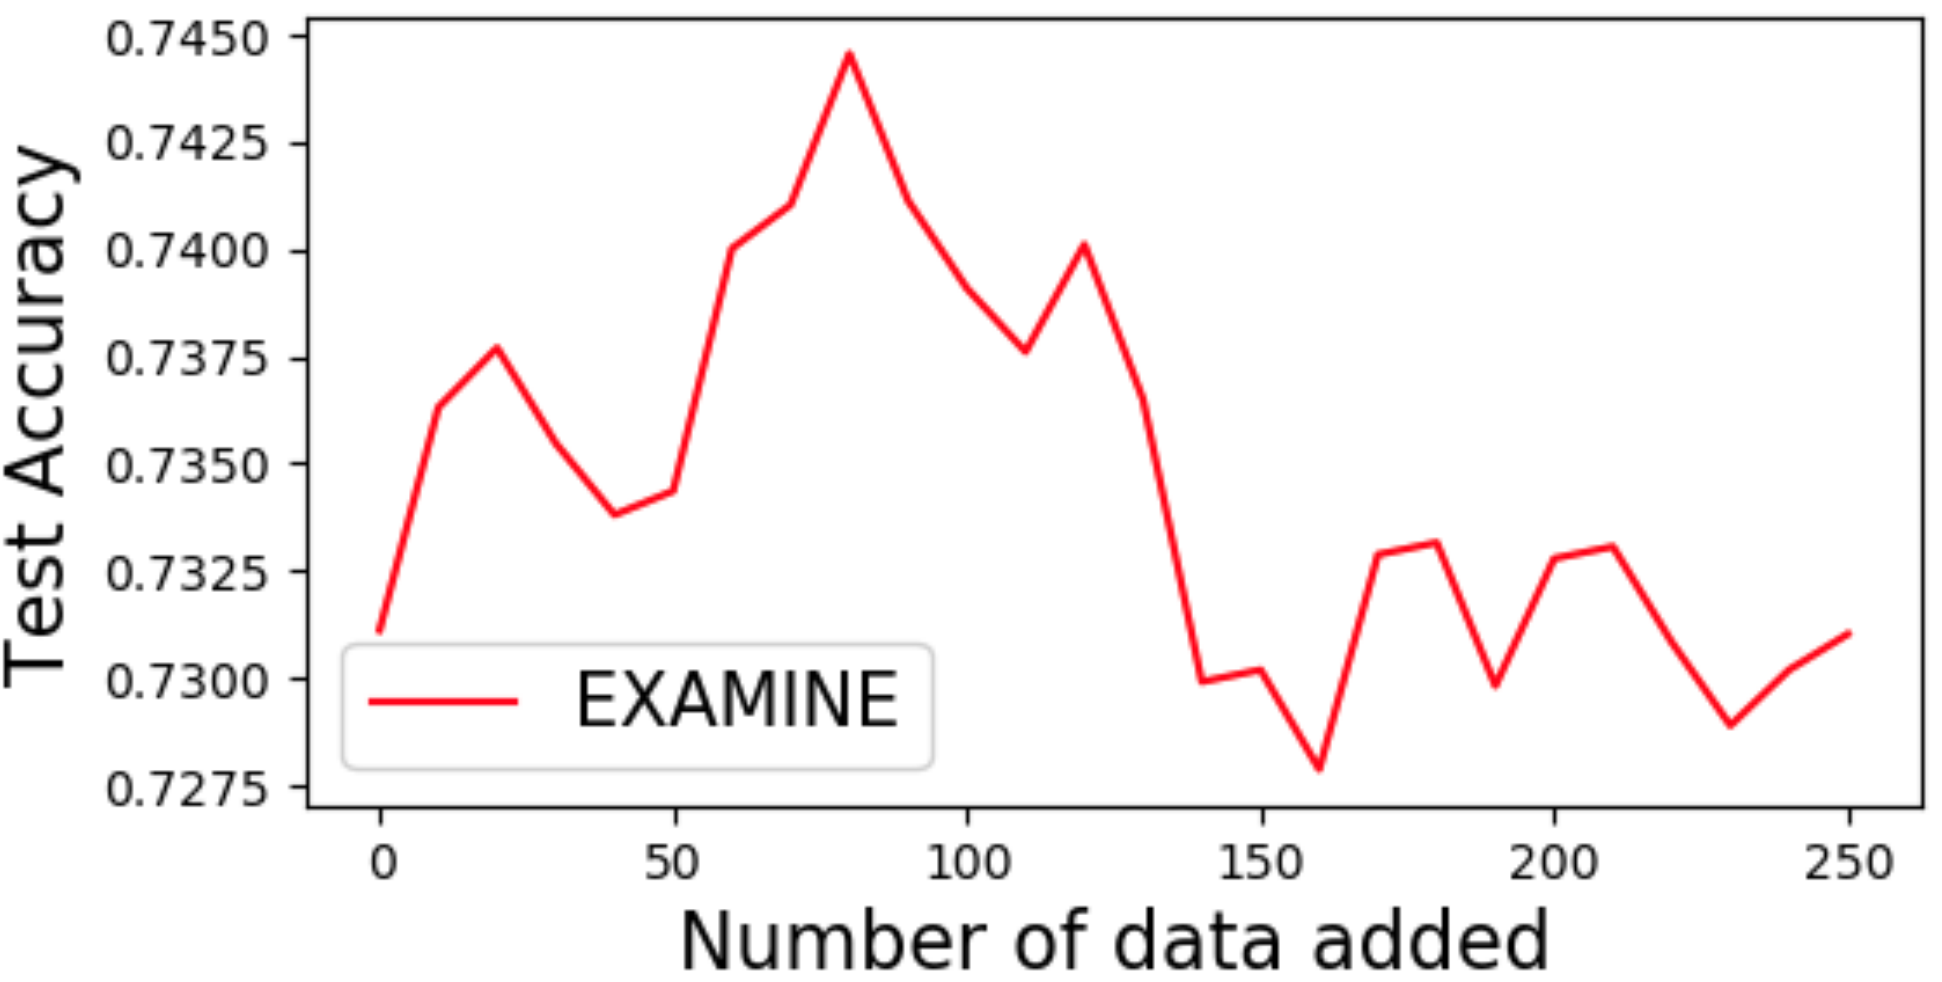}
        \label{fig:covidx_add_bad}
    }\\
    
    \subfloat[Remove high value data]{
        \includegraphics[width=0.47\linewidth]{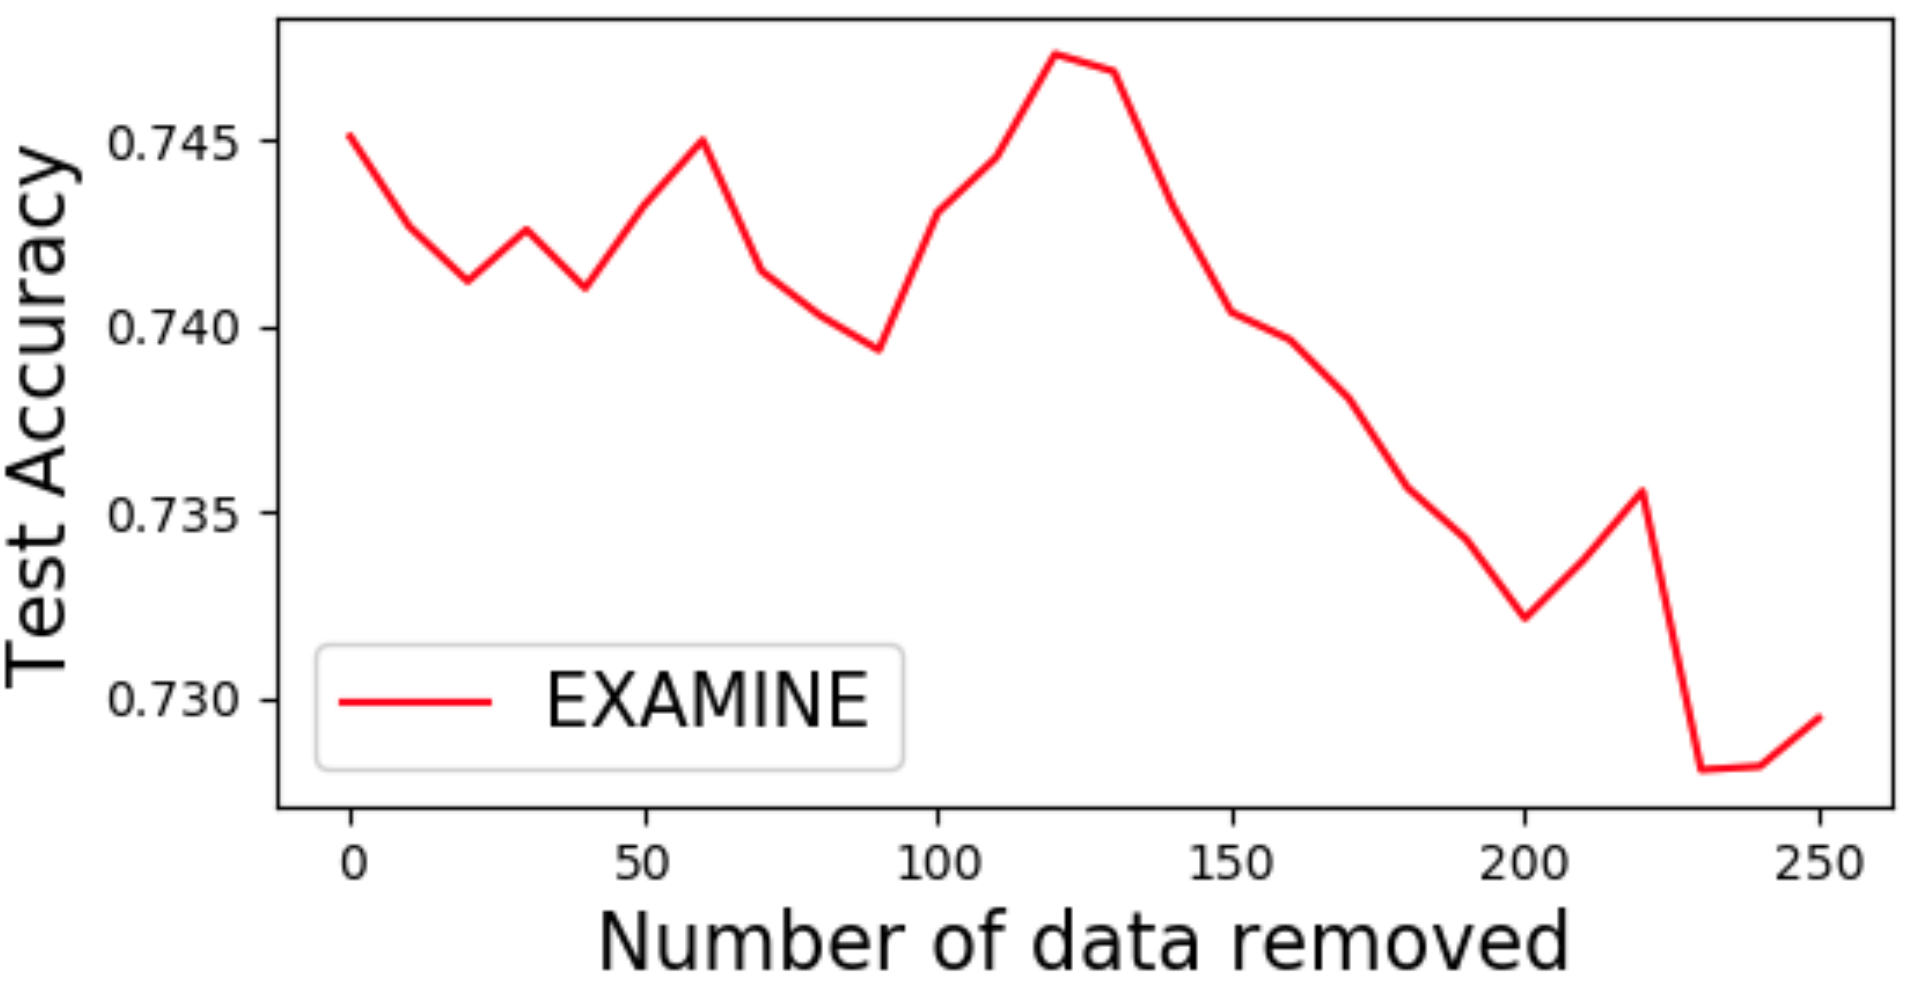}
        \label{fig:covidx_remove_good}
    }
    \subfloat[Remove low value data]{
        \includegraphics[width=0.47\linewidth]{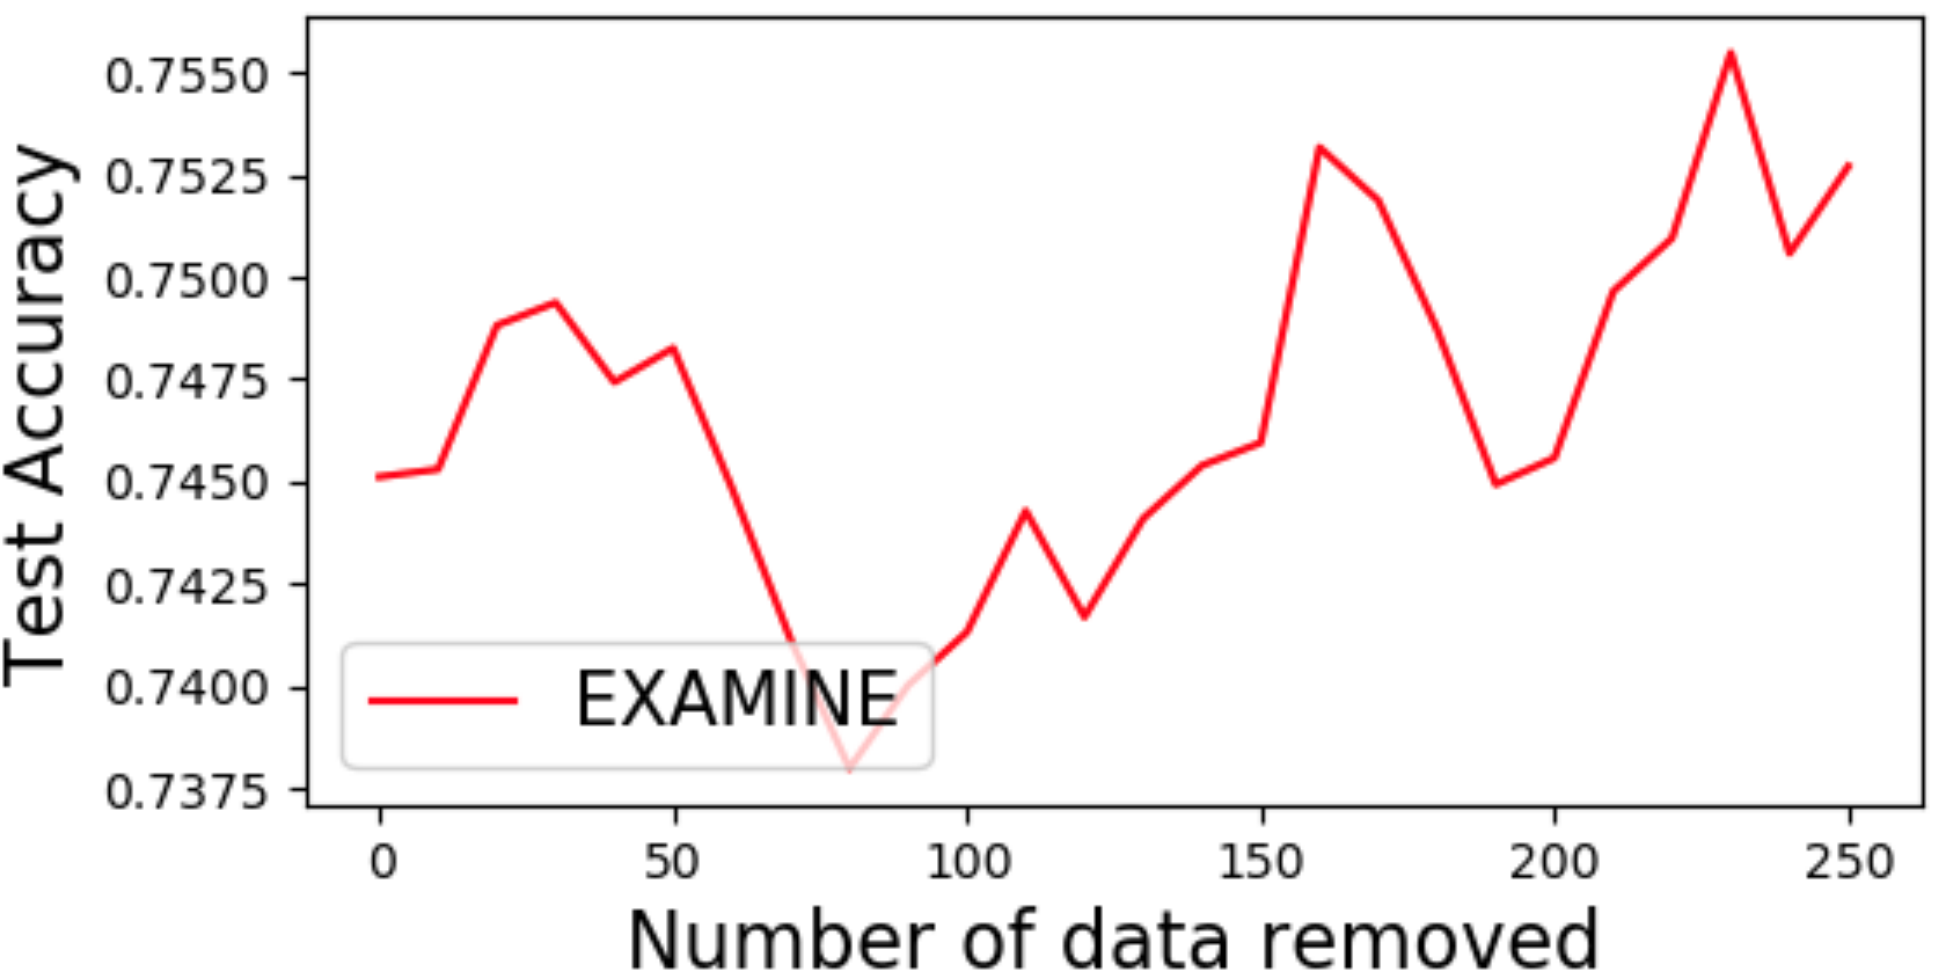}
        \label{fig:covidx_remove_bad}
    }
    
    \caption{We validate \ours{} on COVIDx dataset. We repeated the experiment setting as indicated in Sec.~\ref{exp:data_valuation}. We randomly sample 6,050 data points from each of the two classes, \textit{pneumonia} and \textit{normal} and 500 data unlabeled data points for assessment. The images are resized to 224 $\times$ 224. When training the MAE, we change patch size to 16, masking ratio to $75\%$, and embedded dimension to 512. We uniformly add different levels of Gaussian noise with mean 0 and standard deviation $\sigma = \{0, 0.4, 0.8, 1.2, 1.6\}$ and Gaussian blur with kernel size = $\{0, 9, 17, 25, 33\}$. (a) Adding high value data for training on the descending order of data value results in the sharp increase of accuracy. (b) Adding low value data for training shows an overall decreasing then flattening trend in accuracy. (c) Removing high value data for training leads accuracy drop. %Shapley~\cite{pmlr-v97-ghorbani19c} and LOO~\cite{cook1977detection}. 
    (d) Removing low value data for training yields increase in accuracy.  }
    \label{fig:covidx}
\vspace{-10mm}
\end{figure}

\subsection{Proof Sketch of Theorem~\ref{th:ssl}}

\begin{assumption} \label{assum} Let $X_1 \in \bR^{d_1}, X_2 \in \bR^{d_2}$ be random variables from some unknown distribution. Let $Y \in \mathcal{Y}$ be a discrete random variable with $k = |\mathcal{Y}| < d_2$. We assume conditional independence: $X_1 \perp X_2 | Y$.
\end{assumption}

\noindent \textit{Proof Sketch.} For $X_1, X_2, Y$ satisfy Assumption~\ref{assum}, and $\bA \in \R^{\mathcal{Y}\times d_2}$ with $\bA_{y,:} = \E[X_2|Y = \mathbf{y}]$ has rank $k=|\mathcal{Y}|$. Then
\begin{align*}
    f^*(\cdot) &=\E[X_2|X_1]=\E\left[\E[X_2|X_1,Y]|X_1 \right] = \E\left[\E[X_2|Y]|X_1\right] \\ &= \sum_y P(Y=y|X_1)\E[X_2|Y=y] = h(X_1)^\top \bA
\end{align*}
% $f^*(\cdot)=\E[X_2|X_1]=\E\left[\E[X_2|X_1,Y]|X_1 \right] = \E\left[\E[X_2|Y]|X_1\right] = \sum_y P(Y=y|X_1)\E[X_2|Y=y] = h(X_1)^\top \bA,$
where $f(x_1)_y = P(Y=y|X_1 =x).$ One could see $f^*$ has implicitly encoded the information of $Y|X_1$ given the conditional independence assumption. Finally due to the fact that matrix $\bA$ is full-rank, we get that $h^*$ is linear in $f^*$ as well. 

\subsection{Detailed model architectures}
\begin{table*}[h]
\centering
\caption{MAE model architecture}
\begin{tabular}{|c|cccc|}
\hline
\textbf{Layer}               & \multicolumn{4}{c|}{\textbf{Details}}                                                                                                                                        \\ \hline
\multirow{17}{*}{1} & \multicolumn{1}{c|}{\multirow{17}{*}{Encoder}} & \multicolumn{1}{c|}{Patch Embedding}               & \multicolumn{2}{c|}{Rearrange+Linear}                         \\ \cline{3-5} 
                    & \multicolumn{1}{c|}{}                          & \multicolumn{3}{c|}{Concatenate CLS token}                                                                         \\ \cline{3-5} 
                    & \multicolumn{1}{c|}{}                          & \multicolumn{3}{c|}{Positional Embedding}                                                                          \\ \cline{3-5} 
                    & \multicolumn{1}{c|}{}                          & \multicolumn{3}{c|}{Dropout}                                                                                       \\ \cline{3-5} 
                    & \multicolumn{1}{c|}{}                          & \multicolumn{1}{c|}{\multirow{13}{*}{Transformer}} & \multicolumn{1}{c|}{\multirow{7}{*}{Attention}}   & LayerNorm \\ \cline{5-5} 
                    & \multicolumn{1}{c|}{}                          & \multicolumn{1}{c|}{}                              & \multicolumn{1}{c|}{}                             & Linear    \\ \cline{5-5} 
                    & \multicolumn{1}{c|}{}                          & \multicolumn{1}{c|}{}                              & \multicolumn{1}{c|}{}                             & Matmul    \\ \cline{5-5} 
                    & \multicolumn{1}{c|}{}                          & \multicolumn{1}{c|}{}                              & \multicolumn{1}{c|}{}                             & Softmax   \\ \cline{5-5} 
                    & \multicolumn{1}{c|}{}                          & \multicolumn{1}{c|}{}                              & \multicolumn{1}{c|}{}                             & Matmul    \\ \cline{5-5} 
                    & \multicolumn{1}{c|}{}                          & \multicolumn{1}{c|}{}                              & \multicolumn{1}{c|}{}                             & Linear    \\ \cline{5-5} 
                    & \multicolumn{1}{c|}{}                          & \multicolumn{1}{c|}{}                              & \multicolumn{1}{c|}{}                             & Dropout   \\ \cline{4-5} 
                    & \multicolumn{1}{c|}{}                          & \multicolumn{1}{c|}{}                              & \multicolumn{1}{c|}{\multirow{6}{*}{FeedForward}} & LayerNorm \\ \cline{5-5} 
                    & \multicolumn{1}{c|}{}                          & \multicolumn{1}{c|}{}                              & \multicolumn{1}{c|}{}                             & Linear    \\ \cline{5-5} 
                    & \multicolumn{1}{c|}{}                          & \multicolumn{1}{c|}{}                              & \multicolumn{1}{c|}{}                             & GELU      \\ \cline{5-5} 
                    & \multicolumn{1}{c|}{}                          & \multicolumn{1}{c|}{}                              & \multicolumn{1}{c|}{}                             & Dropout   \\ \cline{5-5} 
                    & \multicolumn{1}{c|}{}                          & \multicolumn{1}{c|}{}                              & \multicolumn{1}{c|}{}                             & Linear    \\ \cline{5-5} 
                    & \multicolumn{1}{c|}{}                          & \multicolumn{1}{c|}{}                              & \multicolumn{1}{c|}{}                             & Dropout   \\ \hline
2                   & \multicolumn{4}{c|}{Linear}                                                                                                                                         \\ \hline
\multirow{14}{*}{3} & \multicolumn{1}{c|}{\multirow{14}{*}{Decoder}} & \multicolumn{1}{c|}{\multirow{13}{*}{Transformer}} & \multicolumn{1}{c|}{\multirow{7}{*}{Attention}}   & LayerNorm \\ \cline{5-5} 
                    & \multicolumn{1}{c|}{}                          & \multicolumn{1}{c|}{}                              & \multicolumn{1}{c|}{}                             & Linear    \\ \cline{5-5} 
                    & \multicolumn{1}{c|}{}                          & \multicolumn{1}{c|}{}                              & \multicolumn{1}{c|}{}                             & Matmul    \\ \cline{5-5} 
                    & \multicolumn{1}{c|}{}                          & \multicolumn{1}{c|}{}                              & \multicolumn{1}{c|}{}                             & Softmax   \\ \cline{5-5} 
                    & \multicolumn{1}{c|}{}                          & \multicolumn{1}{c|}{}                              & \multicolumn{1}{c|}{}                             & Matmul    \\ \cline{5-5} 
                    & \multicolumn{1}{c|}{}                          & \multicolumn{1}{c|}{}                              & \multicolumn{1}{c|}{}                             & Linear    \\ \cline{5-5} 
                    & \multicolumn{1}{c|}{}                          & \multicolumn{1}{c|}{}                              & \multicolumn{1}{c|}{}                             & Dropout   \\ \cline{4-5} 
                    & \multicolumn{1}{c|}{}                          & \multicolumn{1}{c|}{}                              & \multicolumn{1}{c|}{\multirow{6}{*}{FeedForward}} & LayerNorm \\ \cline{5-5} 
                    & \multicolumn{1}{c|}{}                          & \multicolumn{1}{c|}{}                              & \multicolumn{1}{c|}{}                             & Linear    \\ \cline{5-5} 
                    & \multicolumn{1}{c|}{}                          & \multicolumn{1}{c|}{}                              & \multicolumn{1}{c|}{}                             & GELU      \\ \cline{5-5} 
                    & \multicolumn{1}{c|}{}                          & \multicolumn{1}{c|}{}                              & \multicolumn{1}{c|}{}                             & Dropout   \\ \cline{5-5} 
                    & \multicolumn{1}{c|}{}                          & \multicolumn{1}{c|}{}                              & \multicolumn{1}{c|}{}                             & Linear    \\ \cline{5-5} 
                    & \multicolumn{1}{c|}{}                          & \multicolumn{1}{c|}{}                              & \multicolumn{1}{c|}{}                             & Dropout   \\ \cline{3-5} 
                    & \multicolumn{1}{c|}{}                          & \multicolumn{3}{c|}{Linear}                                                                                        \\ \hline
*                   & \multicolumn{4}{c|}{Linear Projection Head}                                                                                                                         \\ \hline
\end{tabular}
\end{table*}
